# Supplementary material for: Generalized Contrastive Optimization of Siamese Networks for Place Recognition
Source: arXiv:2103.06638 source file (2023-04-20)

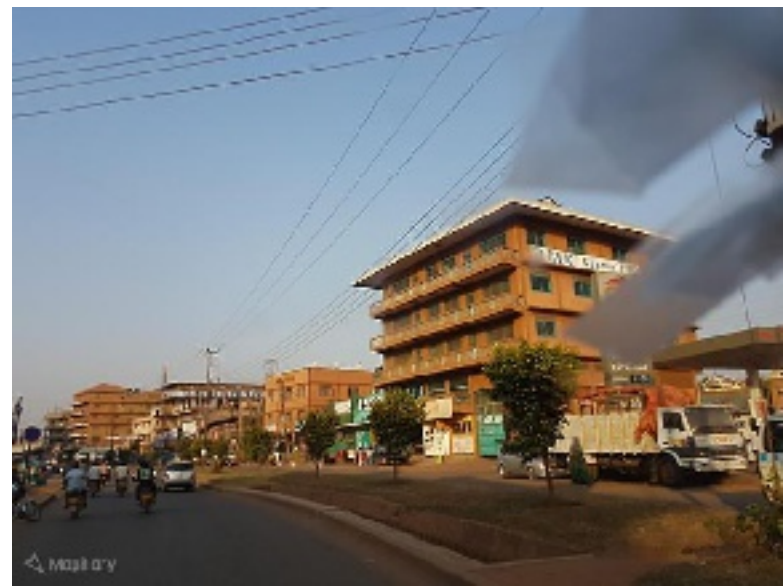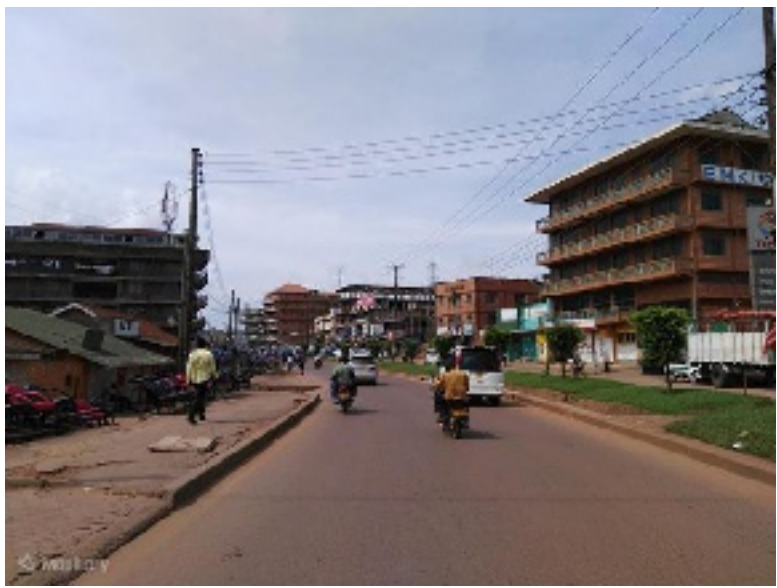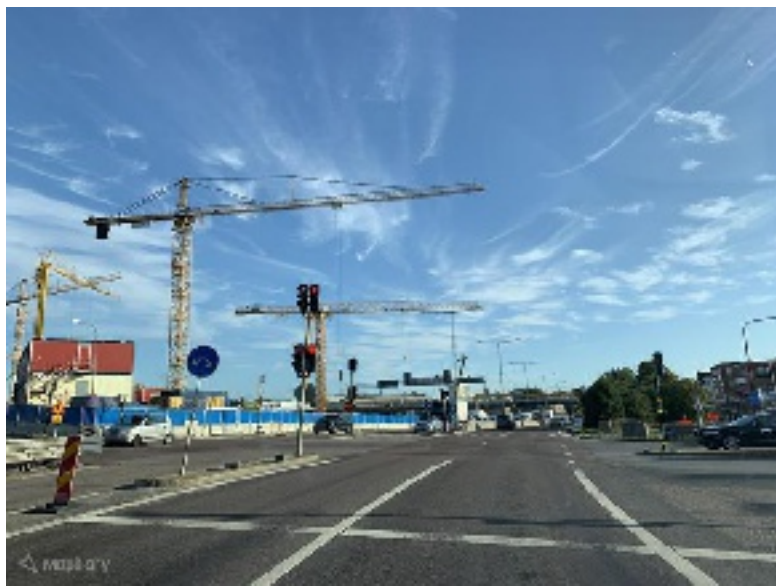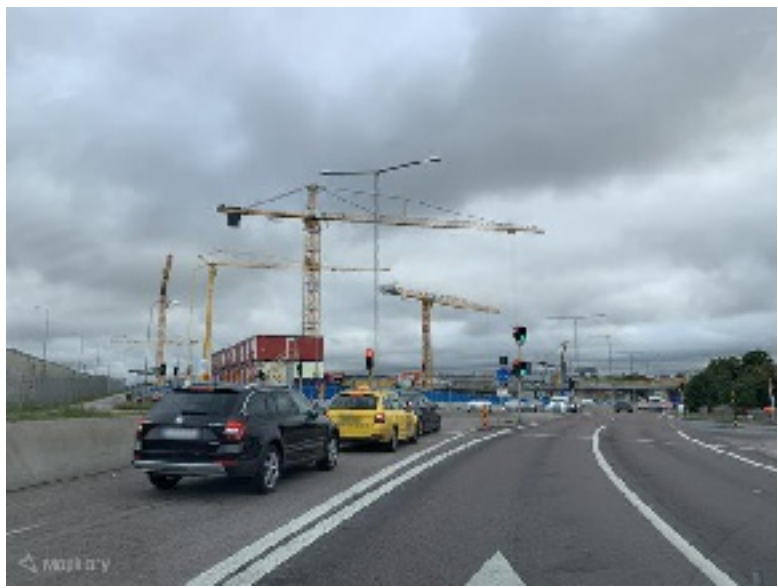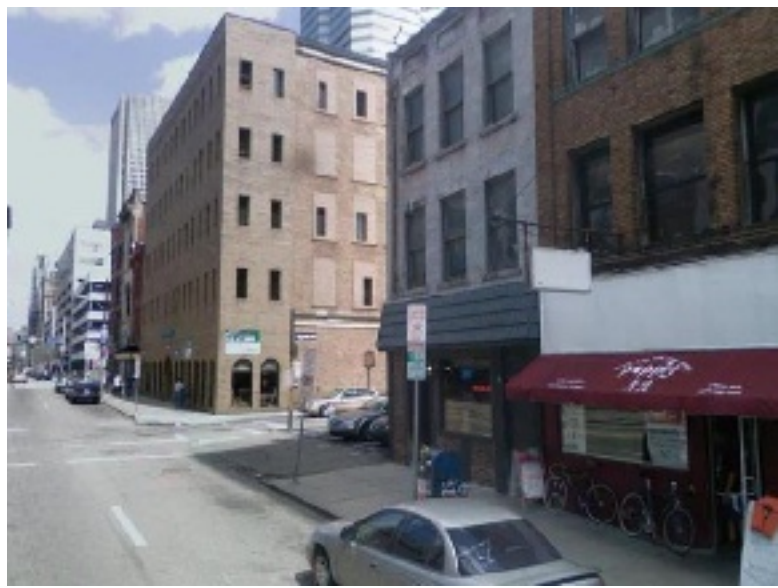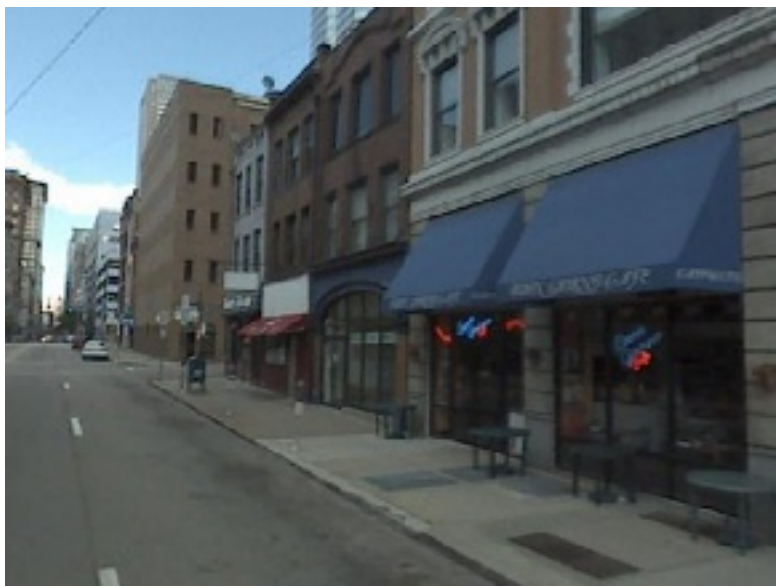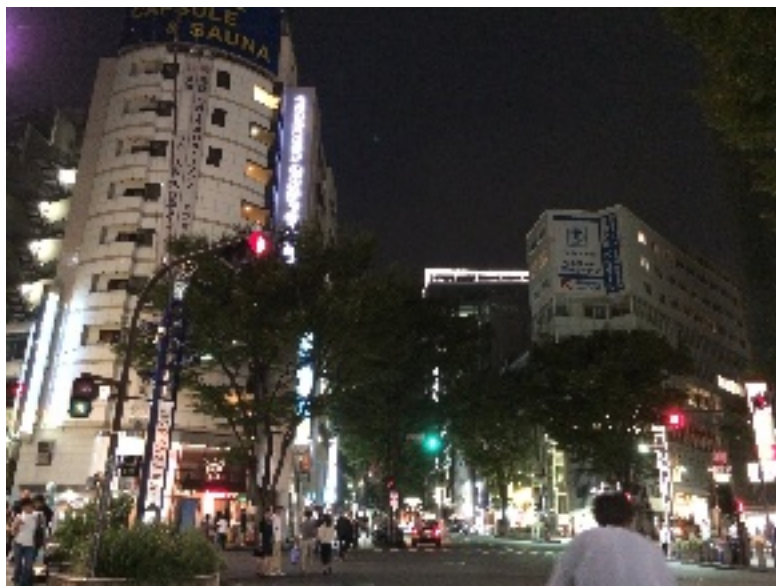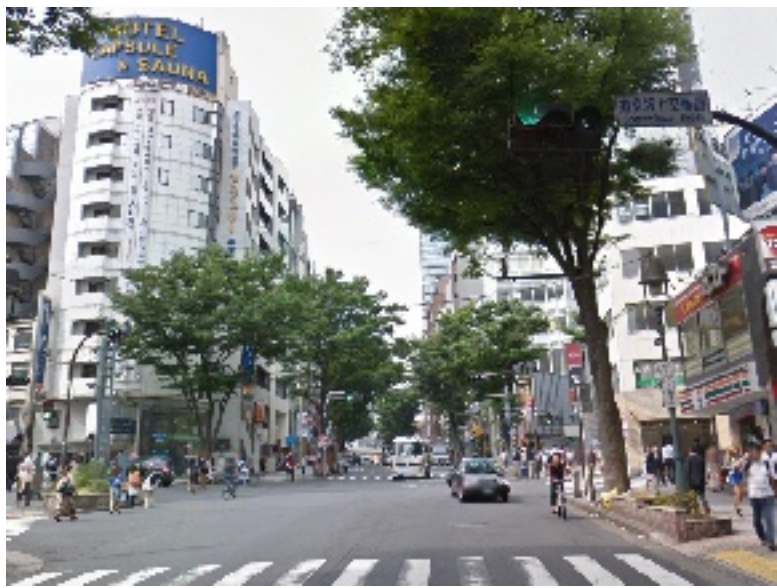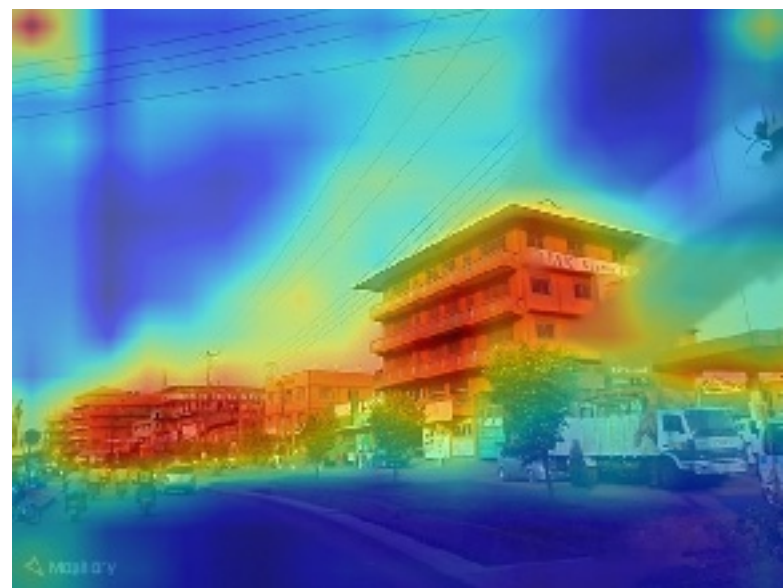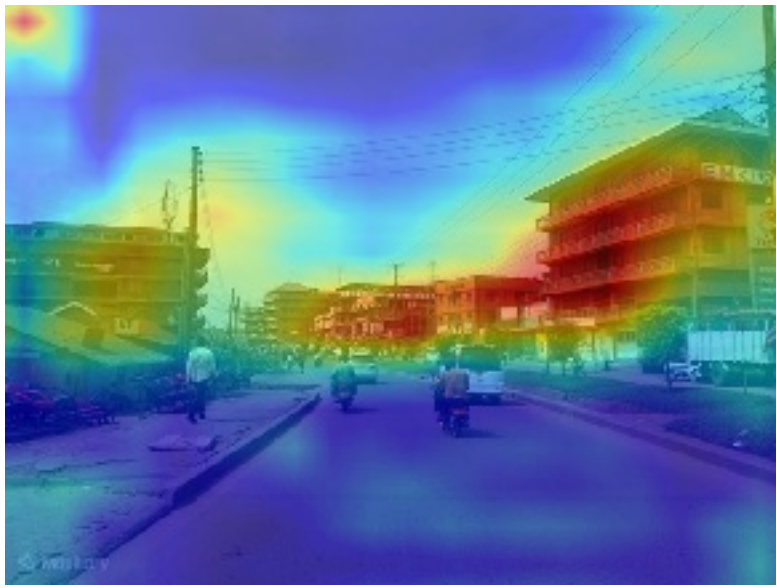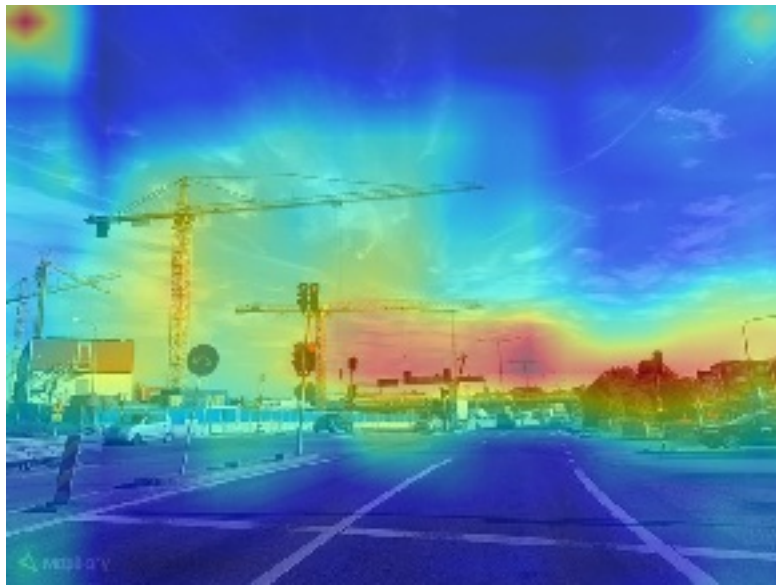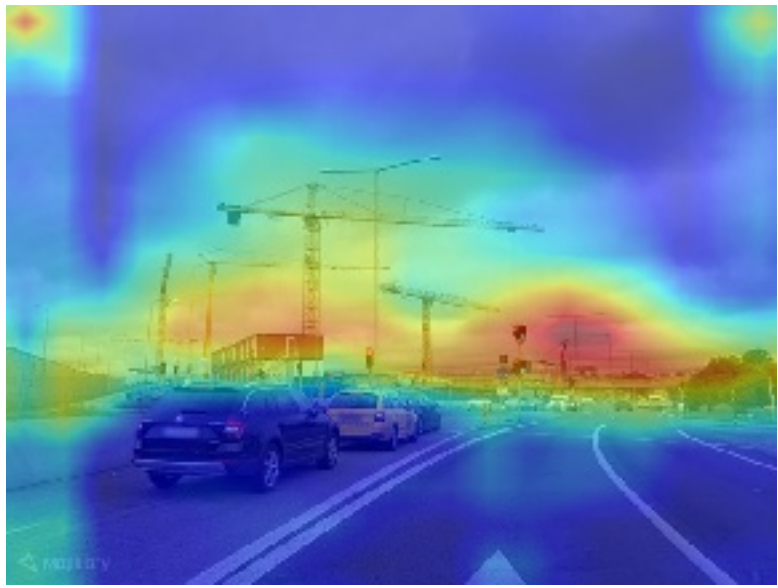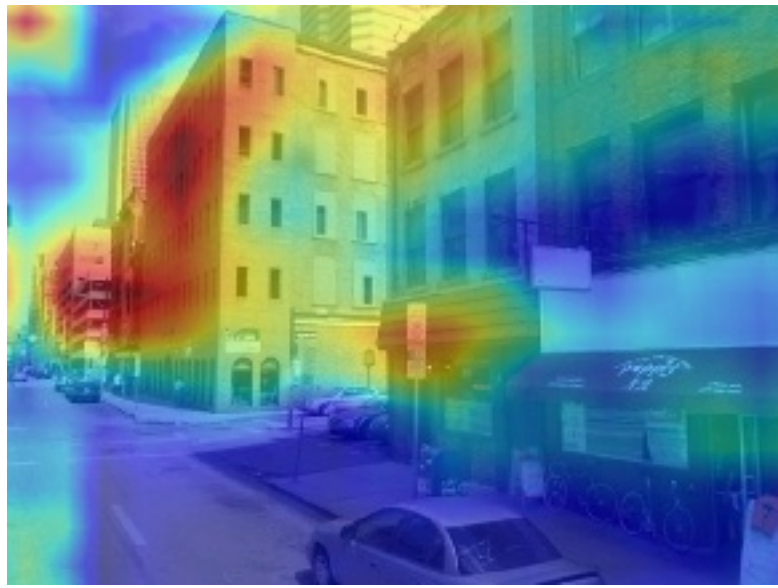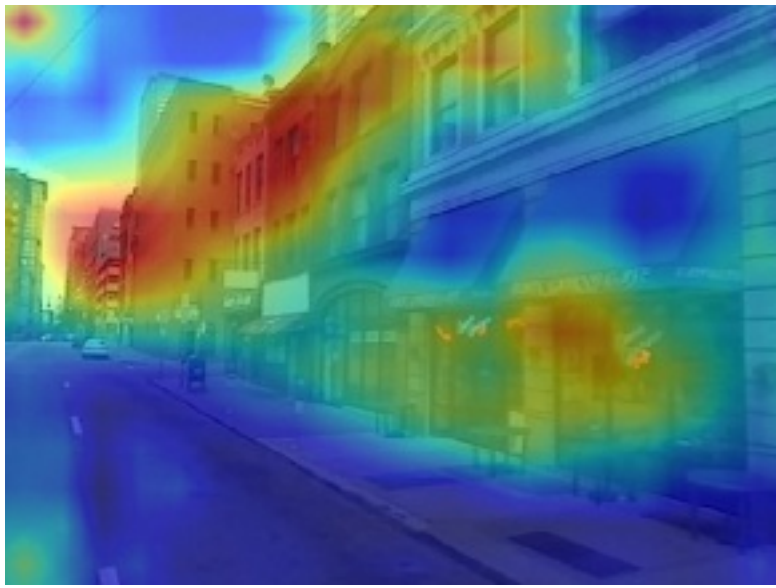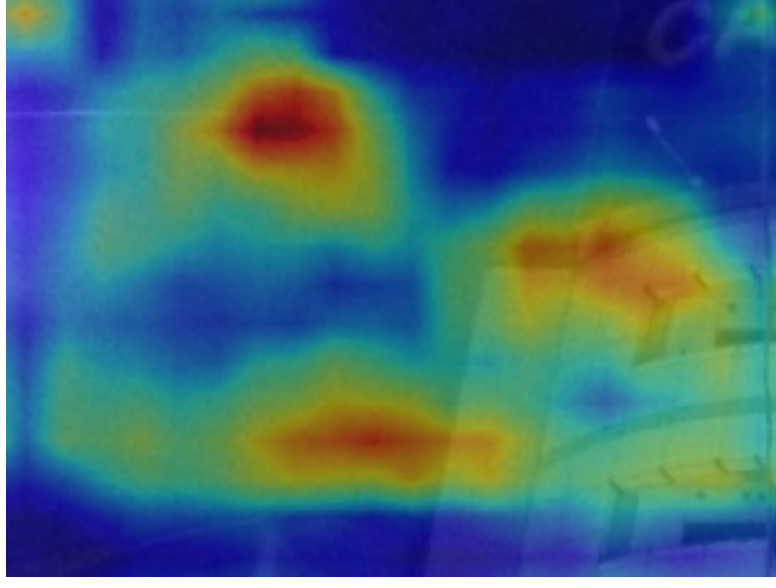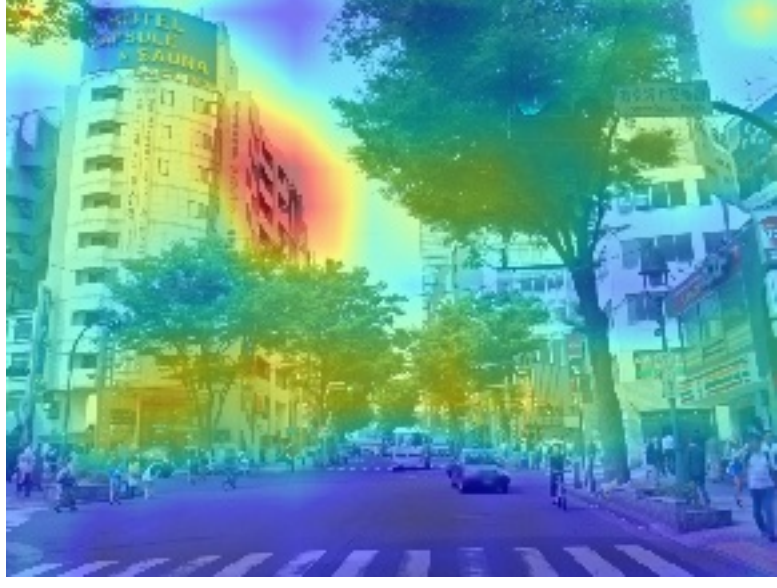



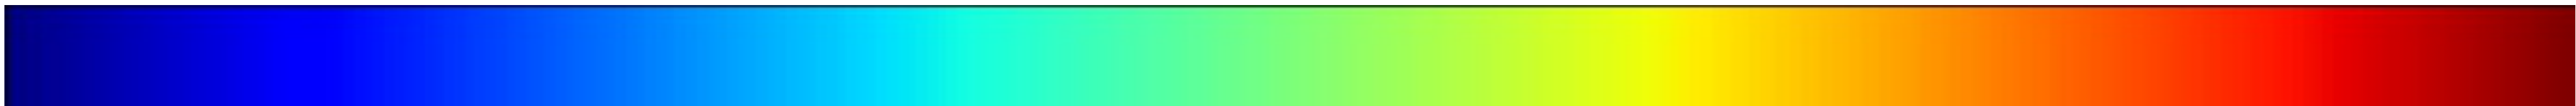



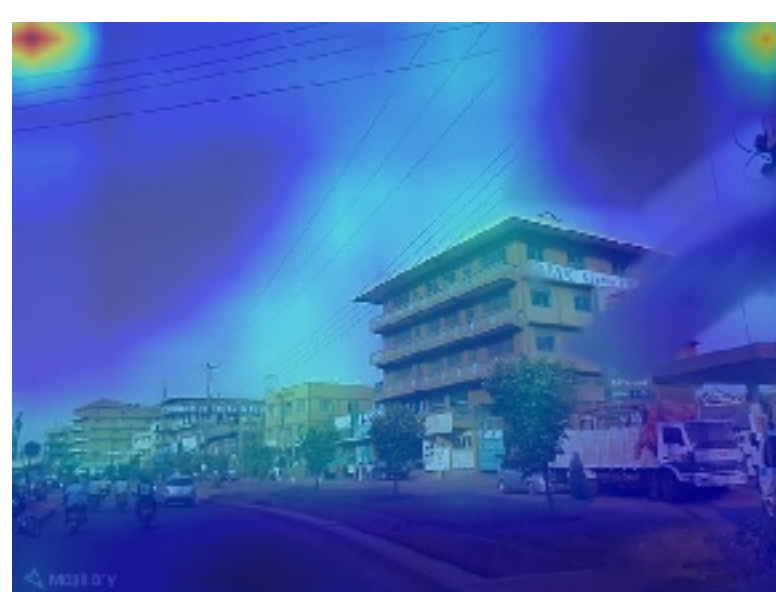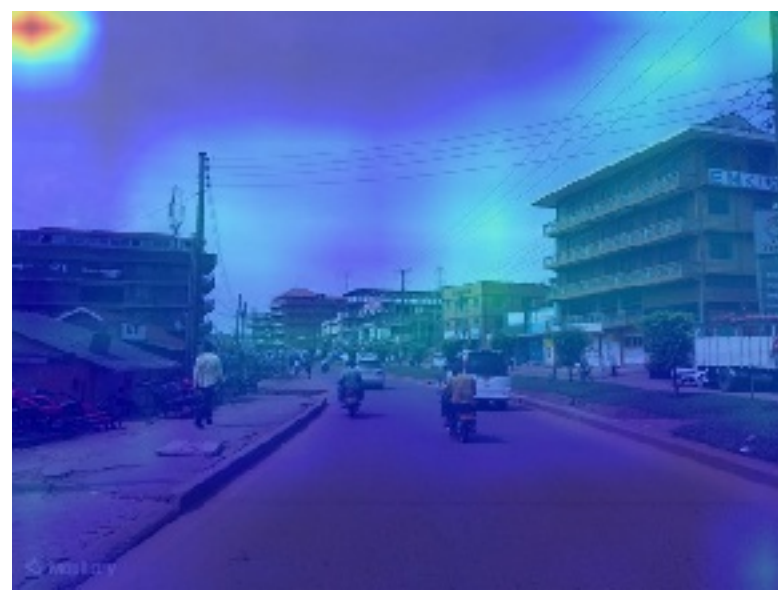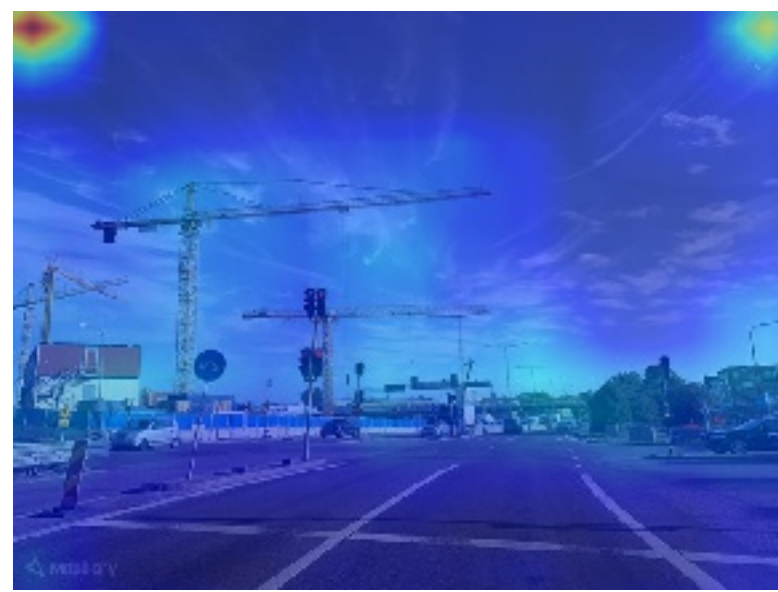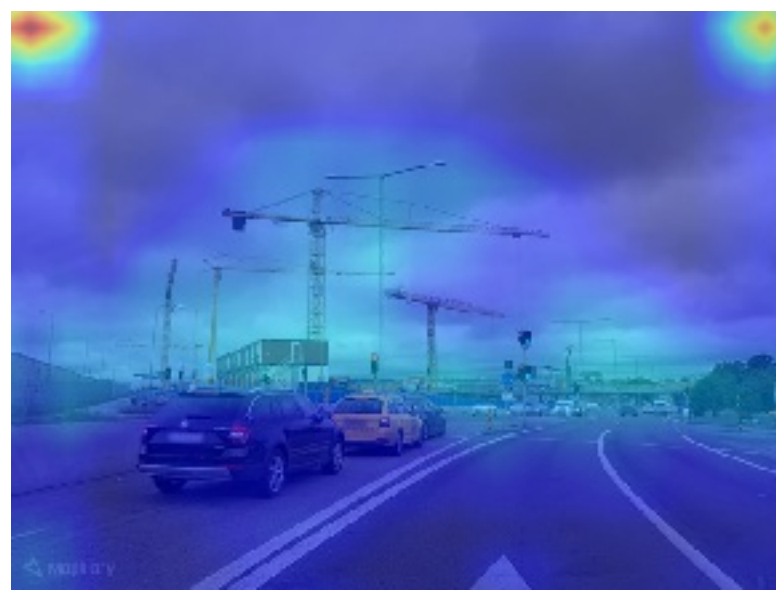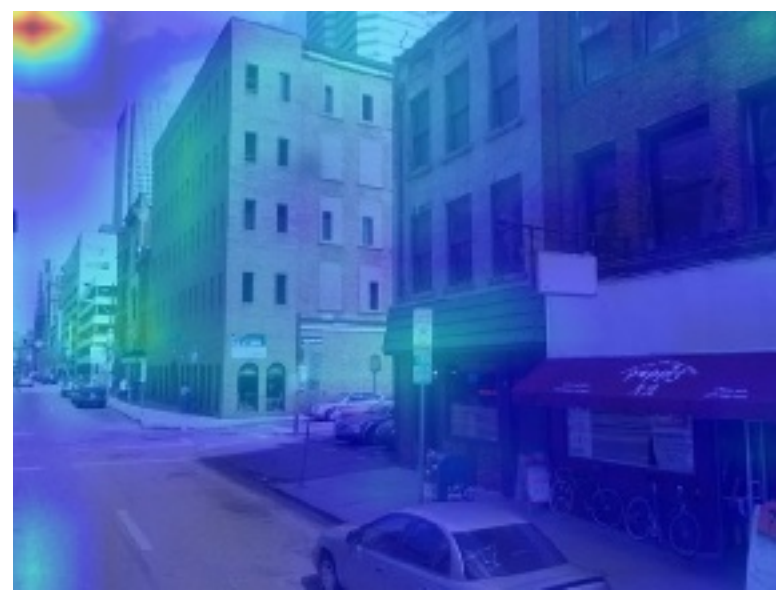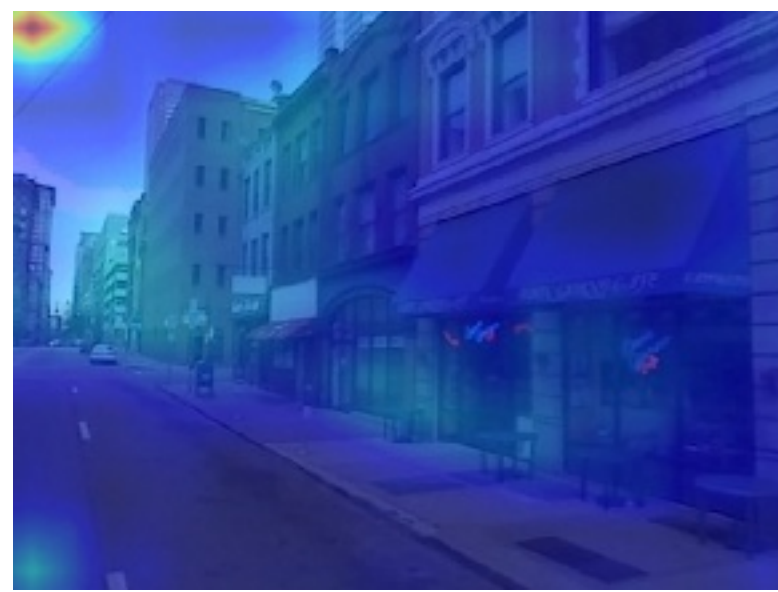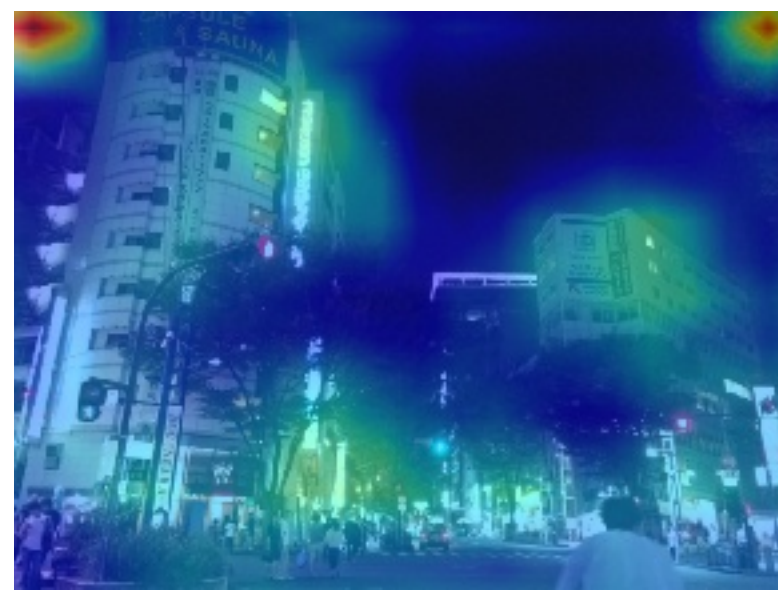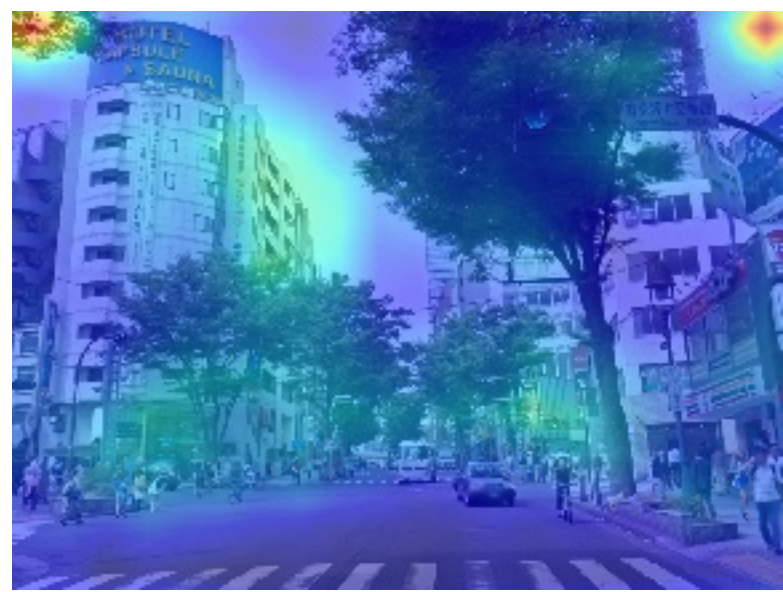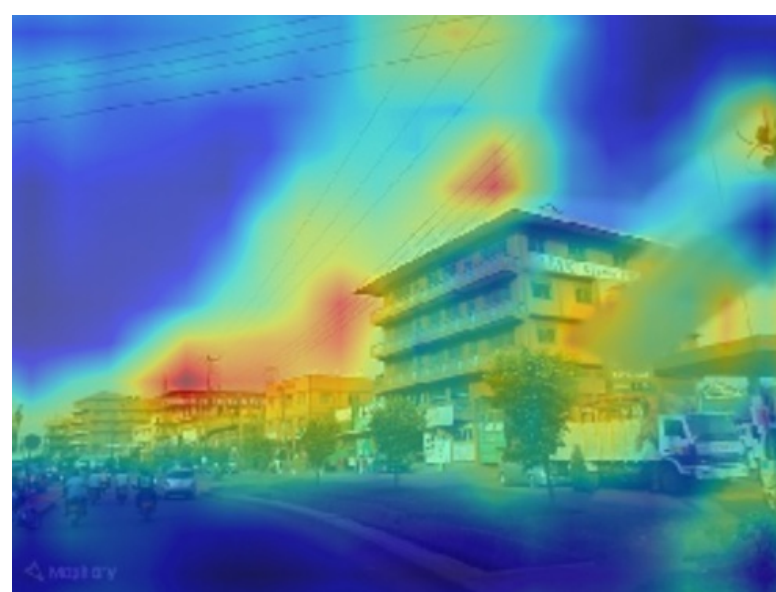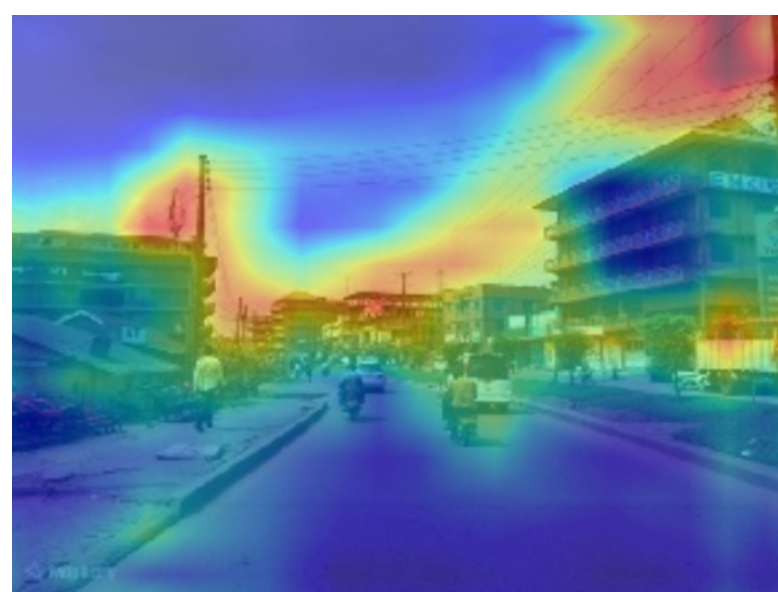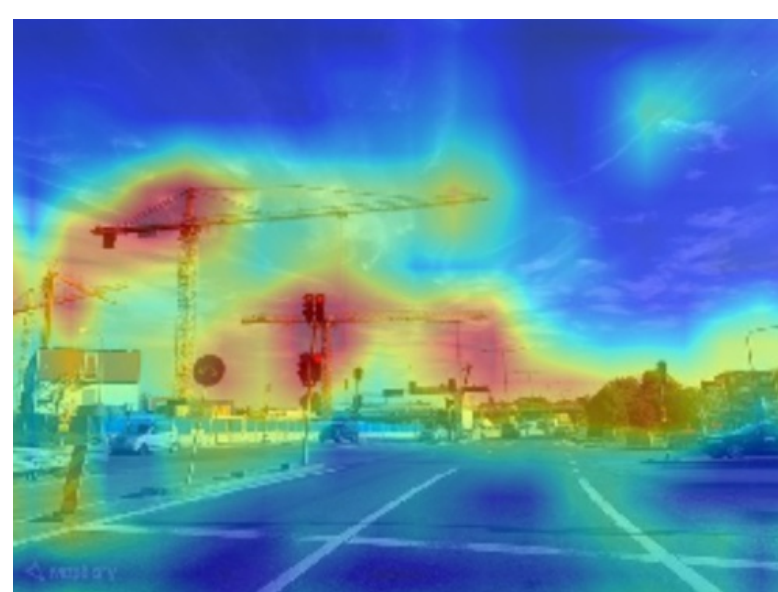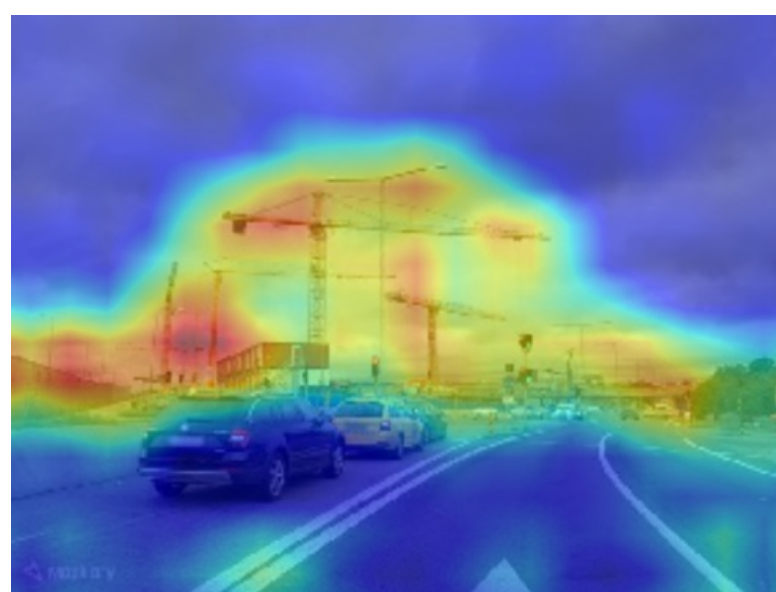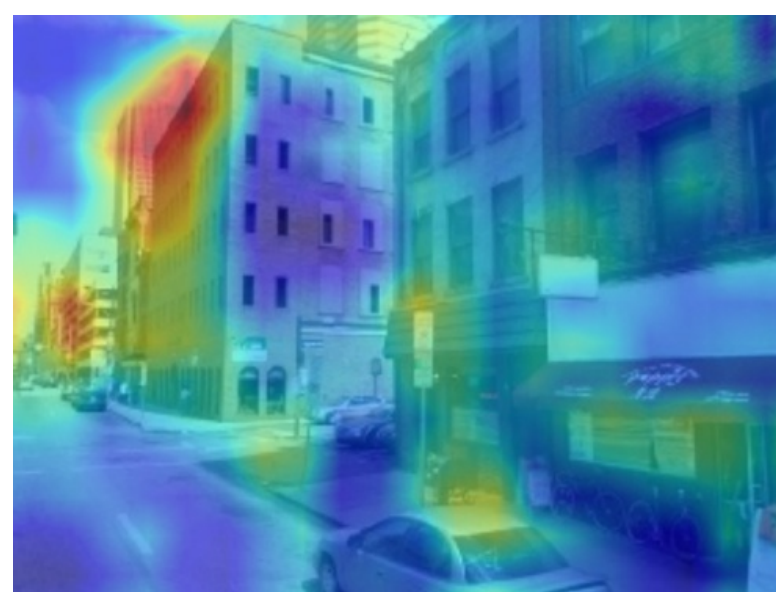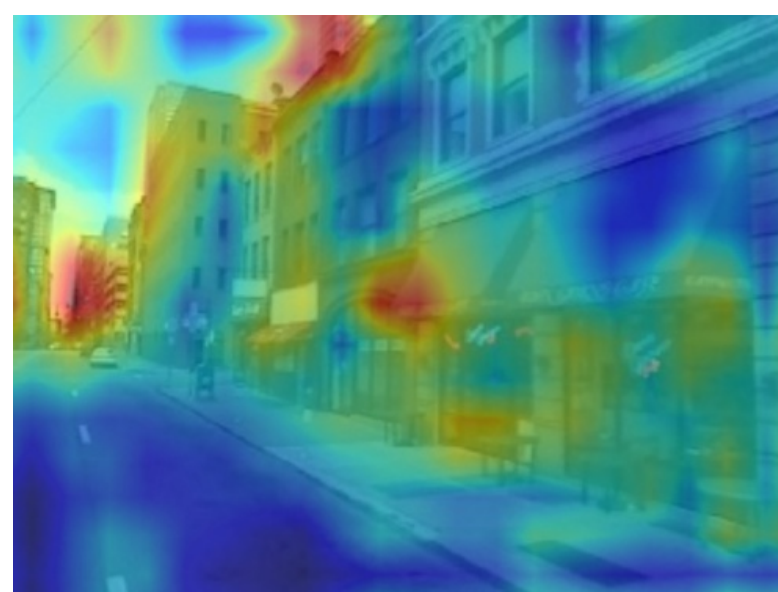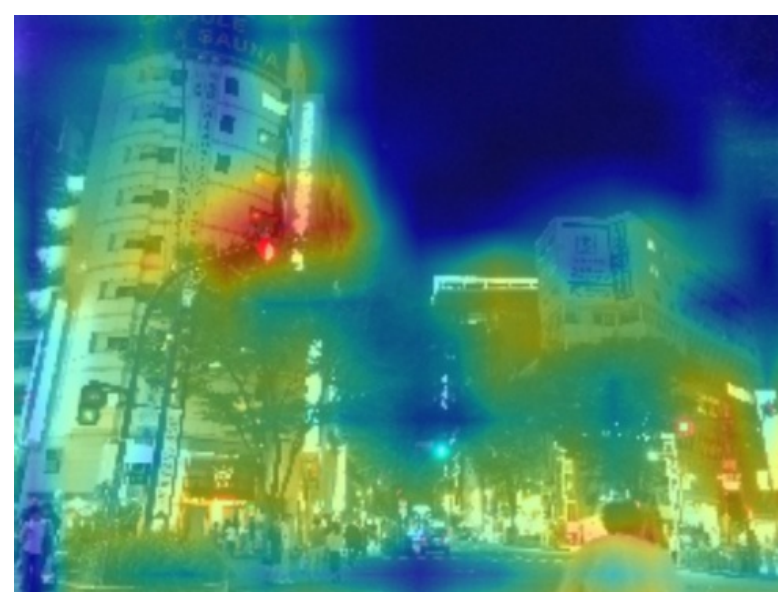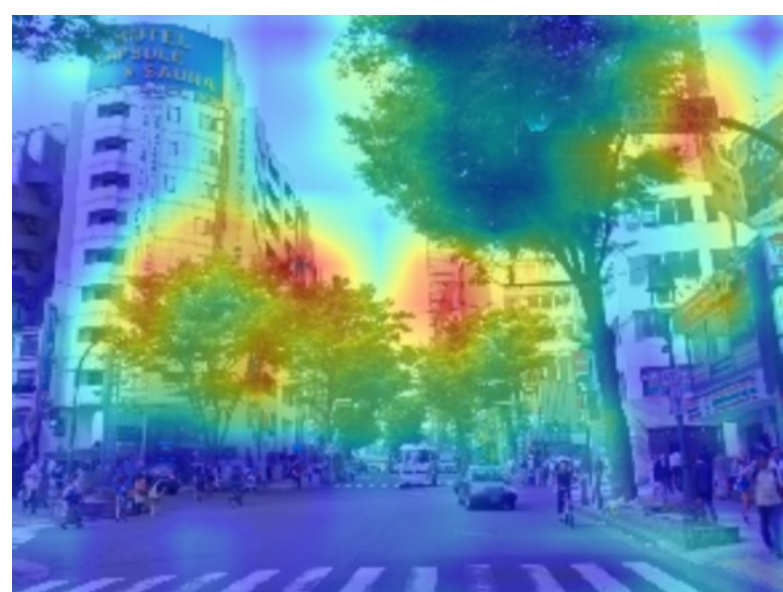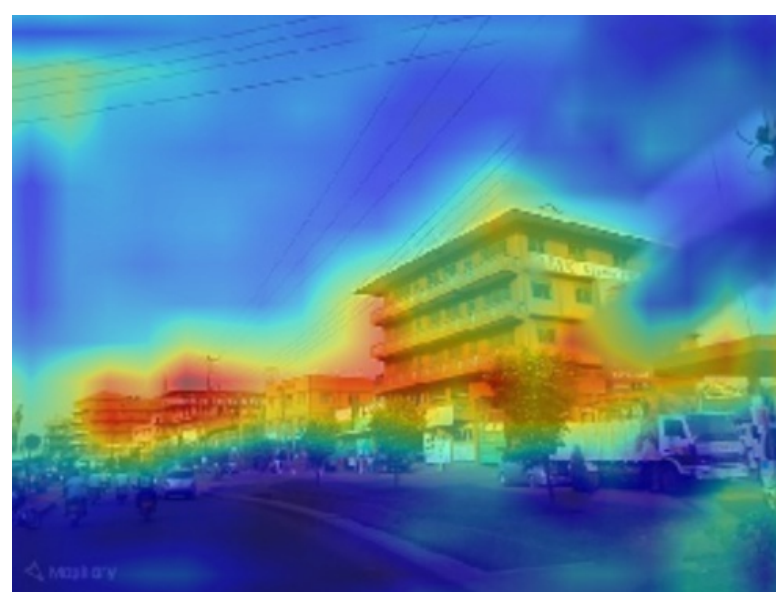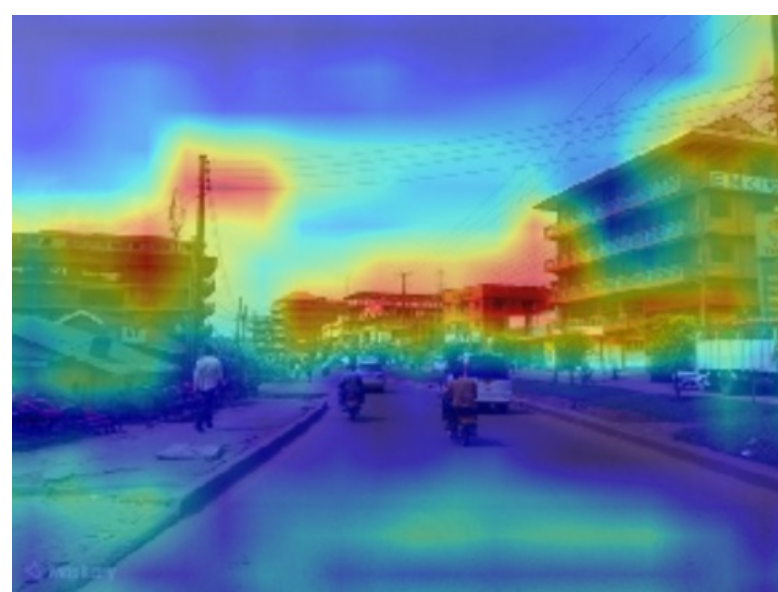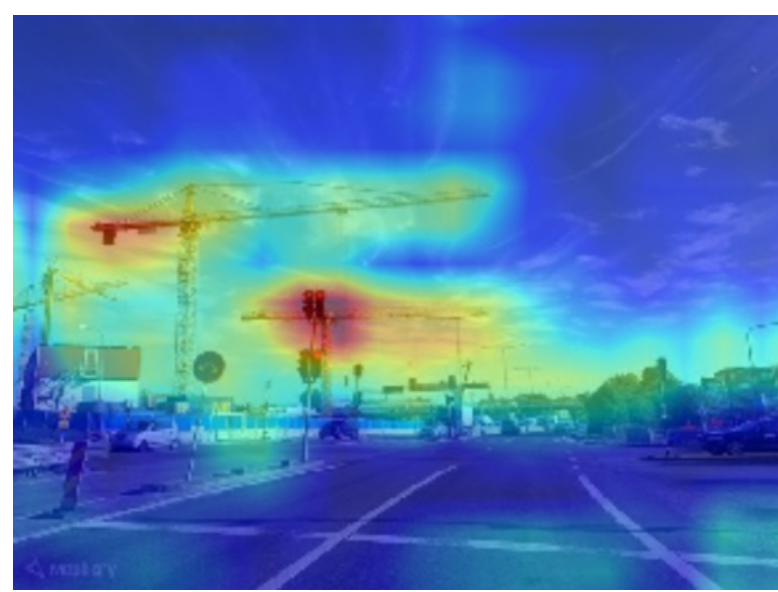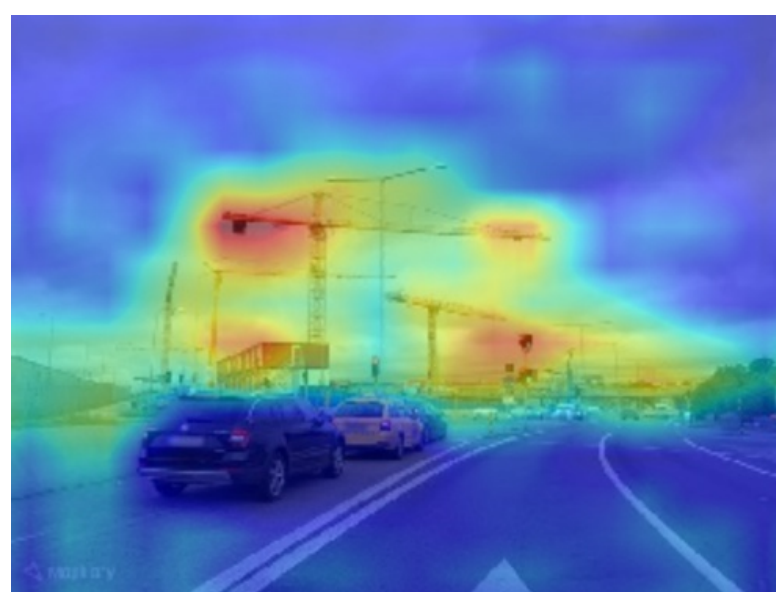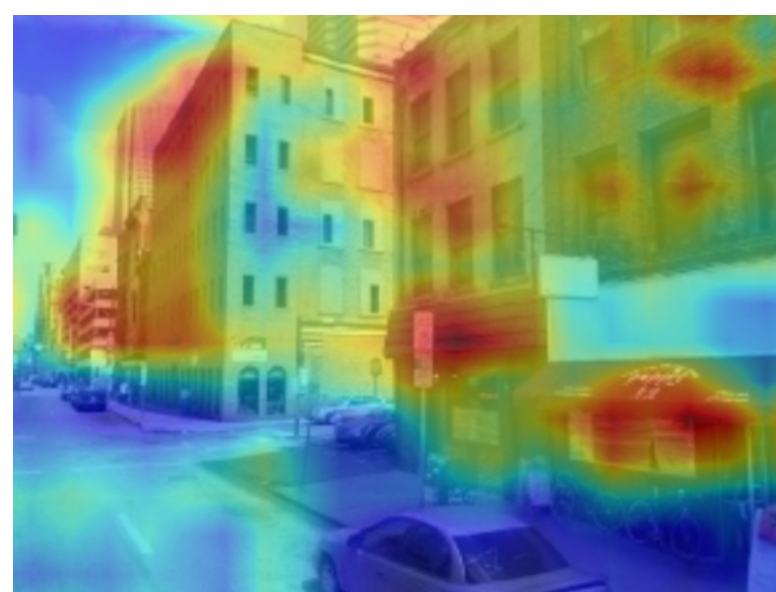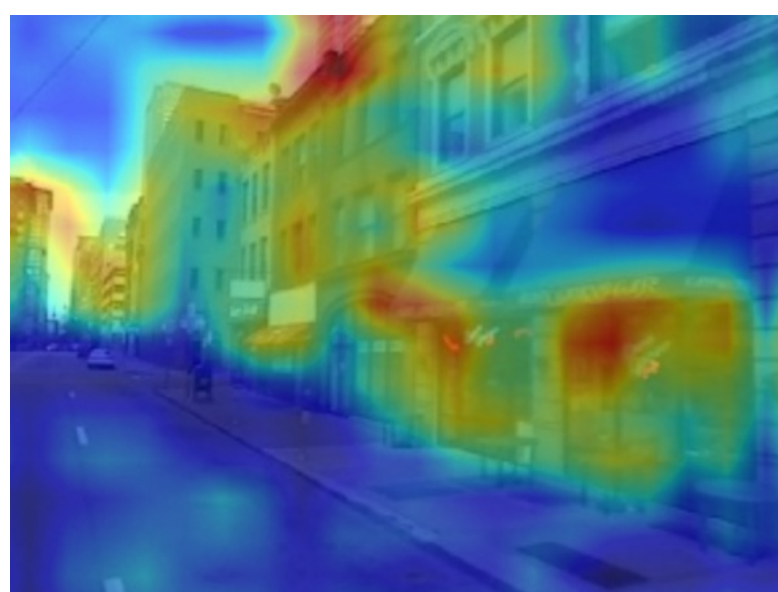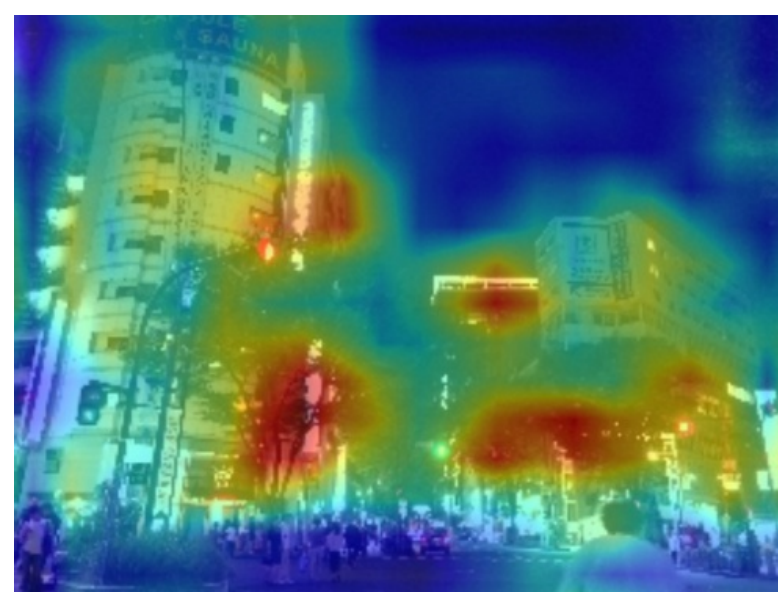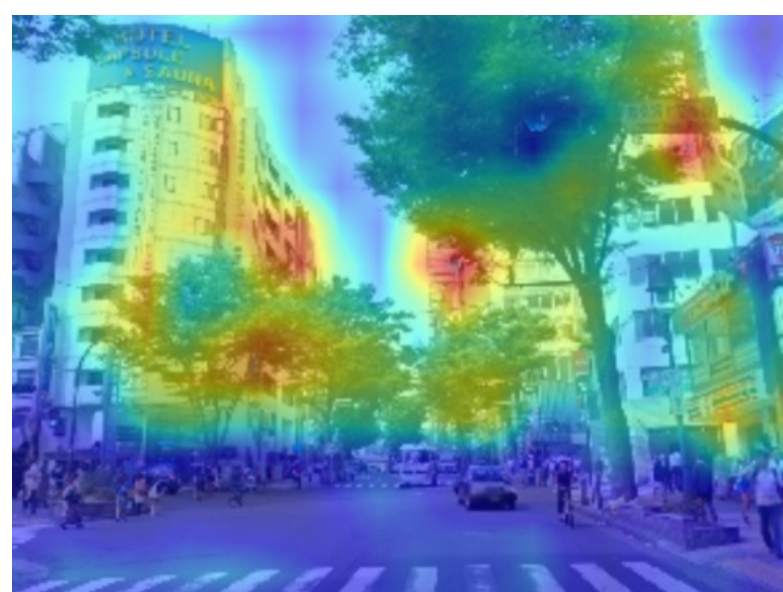

Supplement: Supplementary file 1 [file activations.pdf]
